# Supplementary material for: SuperEdit: Rectifying and Facilitating Supervision for Instruction-Based Image Editing
Source: arXiv:2505.02370 source file (2025-05-05)
Supplement: Supplementary file 1 [file 6_appendix.tex]

\clearpage
\setcounter{page}{1}
\maketitlesupplementary

\section{Overview of Supplementary}
The supplementary material is organized into the following sections:
\begin{itemize}
    \item Section~\ref{supp_human_eval}: Human evaluation.
    \item Section~\ref{supp_diffusion_prior}: More analysis on diffusion generation prior.
    \item Section~\ref{supp_prompt}: Detailed prompt for generation prior.
    \item Section~\ref{supp_analyze_VLM}: Analysis on different vision-language models.
    \item Section~\ref{supp_discussion}: Discussion of broader impact and limitation.
    \item Section~\ref{supp_visualization}: More visualization comparison and results.
\end{itemize}

\section{Human Evaluation}
\label{supp_human_eval}
Following previous methods, we conducted human evaluations on the results of different editing models to thoroughly verify the effectiveness of our method. Specifically, we randomly selected $50$ high-quality, high-resolution images from the MultiReward~\cite{multireward} test dataset. For each image, we used GPT-4o~\cite{gpt4} to generate $7$ different types of editing instructions, including Add, Background Change, Global Change, Local Change, Remove, Style Change, and Material Change. This resulted in a total of $7 \times 50 = 350$ test cases for human evaluation. We then recruited 10 professional annotators to evaluate the edited images based on the three metrics defined in MultiReward~\cite{multireward}, namely, Following, Preserving, and Quality. These metrics assess the degree of execution of the editing instructions, the preservation of non-edited areas of the original image, and the quality of the edited image, respectively. 

We show the human evaluation results in the Table~\ref{tab:human_eval}, our method outperforms all existing methods across all evaluation metrics, indicating that it achieves more precise editing while effectively avoiding modifications to non-editing areas and preventing a degradation in original image quality. For example, we surpass the previous state-of-the-art method, SmartEdit~\cite{smartedit} with the 13B vision-language model (\emph{i.e., LLaVA-13B~\cite{llava}}), in the Following, Preserving, and Quality metrics of human evaluations by 1.80\%, 16.00\%, and 14.80\%, respectively. Please note that our model architecture is fully consistent with InstructPix2Pix~\cite{instruct_p2p}, with no additional parameters introduced.

\begin{table}[th!]
\caption{Human evaluation results on Real-Edit~\cite{multireward} benchmark. All the human evaluated scores are range from 0 to 5. Overall represents the average score of Following, Preserving, and Quality.}
% \vspace{-0.3cm}
\label{tab:human_eval}
\resizebox{\linewidth}{!}{
\begin{tabular}{lllll}
\specialrule{1.5pt}{0pt}{0pt}
 & Following $\uparrow$ & Preserving $\uparrow$ & Quality $\uparrow$ & Overall $\uparrow$ \\
 \hline
InstructPix2Pix~\cite{instruct_p2p} & 2.41 & 2.62 & 2.44 & 2.49 \\
SmartEdit-13B~\cite{smartedit} & 3.09 & 3.06 & 2.63 & 2.93 \\
Ours & \textbf{3.18\textsubscript{\textcolor{red}{\textbf{+1.80\%}}}} & \textbf{3.86\textsubscript{\textcolor{red}{\textbf{+16.00\%}}}} & \textbf{3.37\textsubscript{\textcolor{red}{\textbf{+14.80\%}}}} & \textbf{3.47\textsubscript{\textcolor{red}{\textbf{+10.80\%}}}}
\\ \specialrule{1.5pt}{0pt}{0pt}
\end{tabular}
}
\vspace{-0.5cm}
\end{table}

\section{Diffusion Generation Prior (More Examples)}
\vspace{-0.2cm}
\label{supp_diffusion_prior}
As discussed in the Section 3.2 and Figure 4 of the main paper, editing diffusion models focus on specific generation attributes during inference, independent of the different editing instructions. Specifically, editing models focus on \textbf{global layout} in the early stages, \textbf{local object attributes} in the mid stages, \textbf{image details} in the late stages, and \textbf{style change} of all sampling stages. In this section, we further demonstrate this generation prior in Figure~\ref{fig:supp_diffusion_prior}.

\begin{figure*}[t!]\centering
    \includegraphics[width=1.0\linewidth]{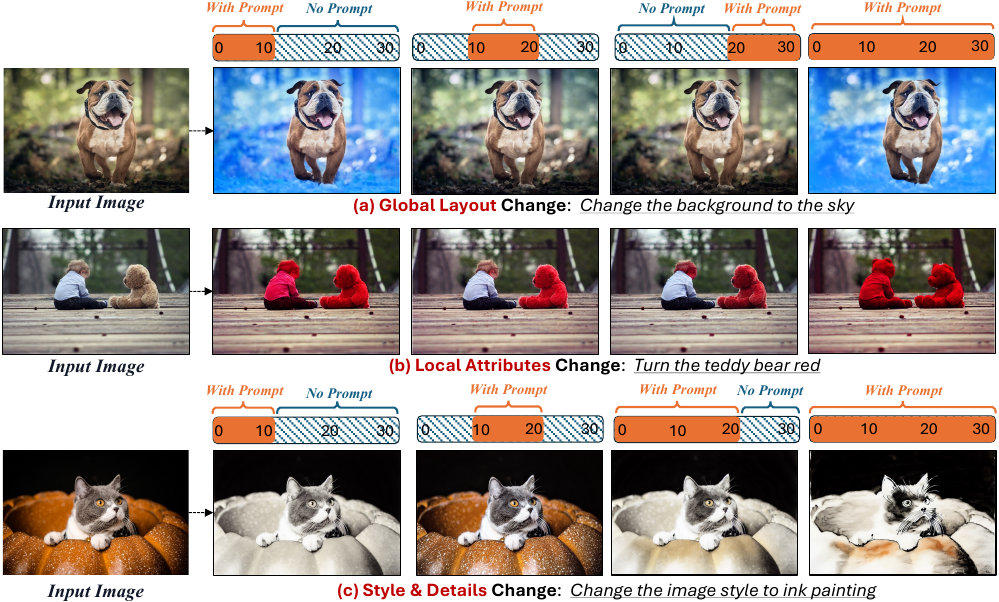}
    \vspace{-0.8cm}
    \caption{
    We show the impact of incorporating the editing prompt at different inference timesteps on the edited image. \textbf{(a)} The global layout changes usually occur in the early stages of inference. Adding text editing instructions to modify the global layout at the mid or late stages does not effectively impact the global layout. \textbf{(b)} Local object attribute changes occur in the mid-stages of sampling. Adding text editing instructions in the early or late stages may result in incorrect editing outcomes. \textbf{(c)} The style changes happen across all inference stages, and the details changes happen in the late stage (Please refer to the subtle differences between the last two images). Best viewed in color.
    }
    \label{fig:supp_diffusion_prior}
\end{figure*}

% \clearpage
\section{GPT-4o Prompts for Constructing Rectified and Contrastive Editing Instructions}
\label{supp_prompt}
\vspace{-0.2cm}
% \paragraph{Prompt for Instruction Rectification.}
We show the detailed prompt for GPT-4o to construct the rectified and contrastive editing instructions in Figure~\ref{fig:gpt_prompts}.
As discussed in Section~\ref{supp_diffusion_prior}, we input the original image and the edited image into GPT-4o and ask it to return the differences in the following four attributes: ``Overall Image Layout ``Local Object Attributes", ``Image Details", and ``Style Change". When calling the GPT-4o API, we explicitly define ``Overall Image Layout" as modifications to the major objects, characters, and background in the image. ``Local Object Attributes" are defined as changes in the texture, motion, pose, and shape of the major objects, characters, and background. Additionally, we combine ``Style" and ``Details" into a single category to reduce the number of tokens generated by GPT-4o, thus saving costs. We observed that this adjustment does not reduce GPT-4o's understanding of the style and detail changes between the original-edited image pair. In the actual training of the editing model, acknowledging that CLIP~\cite{clip} text encoder can accept a maximum of 77 textual tokens as input, we ask GPT-4o to summarize and refine these rectified instructions. We then use the consolidated and refined editing instructions (``Summarized Instruction" in Figure~\ref{fig:gpt_prompts}) to train the model.

\section{Analysis on Different Vision-Language Models.}
\vspace{-0.1cm}
\label{supp_analyze_VLM}
In this section, we investigate existing vision-language models~\cite{llava-ov,llava_next_interleave,gpt4,internvl,gemini} that support multi-image input and understanding. We evaluate these models' ability to describe the differences between input image pairs with the predefined generation priors, as illustrated in the Figure~\ref{fig:supp_vlms}. We find that GPT-4o consistently outputs more accurate and human-perception-aligned editing instructions for various original-edited image pair inputs. In Figure~\ref{fig:supp_recaption_no_prior}, we show that if the predefined four generation prior attributes are not used as in-context learning templates, the GPT-4o rectified editing instructions will contain redundant information and lack the necessary standardization when scaling-up data.

\section{Discussion and Social Impact}
\label{supp_discussion}
\vspace{-0.2cm}
\paragraph{Discussion and Limitation.}
Our method significantly enhances instruction-based image editing but still has limitations. The model struggles with comprehending and executing complex instructions, particularly in images with densely packed objects and intricate spatial relationships. While we use rectified instructions and contrastive supervision signals, inconsistencies may still arise due to the inherent limitations of diffusion models and the challenges of fully capturing natural language nuances. Moreover, ensuring the accuracy and validity of rectified and contrastive instructions requires using GPT-4o~\cite{gpt4}, which may incur additional costs as data volumes scale up.

\vspace{-0.2cm}
\paragraph{Social Impact.}
Advancements in instruction-based image editing bring both positive and negative social impacts. On the positive side, they enhance creative industries, such as graphic design, advertising, entertainment, and education, by providing intuitive tools for content creators. However, these capabilities can also be misused to create deceptive content, such as deepfakes or fake news, raising concerns about privacy, security, and public trust.

\section{More Visualization Comparison and Results}
\label{supp_visualization}
We show more visual comparison with existing instruction-based image editing methods in Figure~\ref{fig:supp_visual_comparison}. Compared to existing instruction-based editing methods, our approach not only better understands and executes editing instructions but also preserves the original image’s layout and quality more effectively, thereby significantly outperforming previous methods.

\begin{figure*}[t!]\centering
    \includegraphics[width=0.9\linewidth]{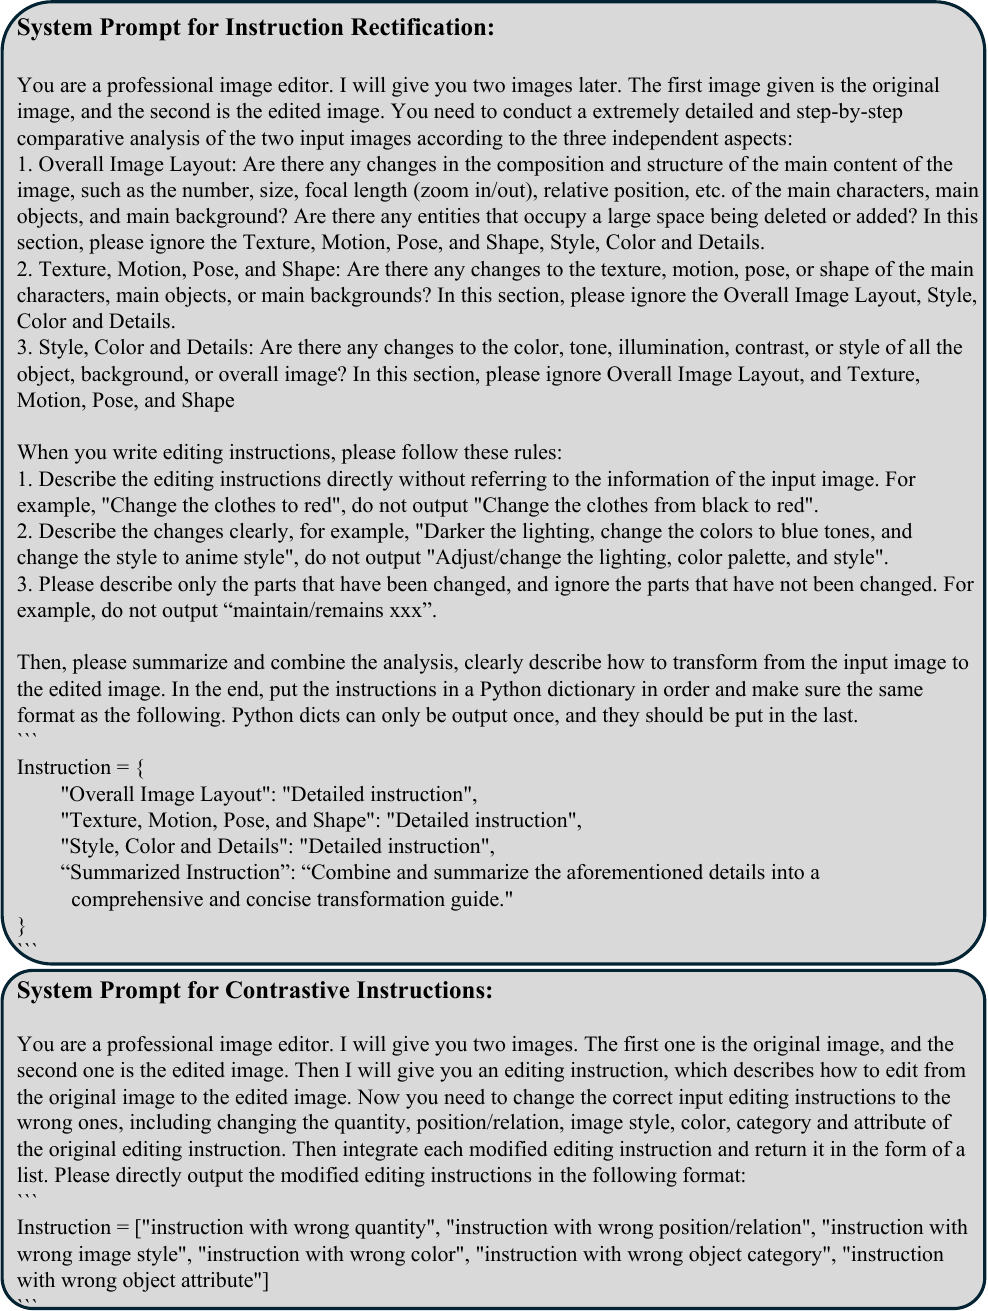}
    \caption{
    GPT-4o prompts for constructing rectified and contrastive editing instructions
    }
    \label{fig:gpt_prompts}
\end{figure*}

\begin{figure*}[t!]\centering
    \includegraphics[width=1.0\linewidth]{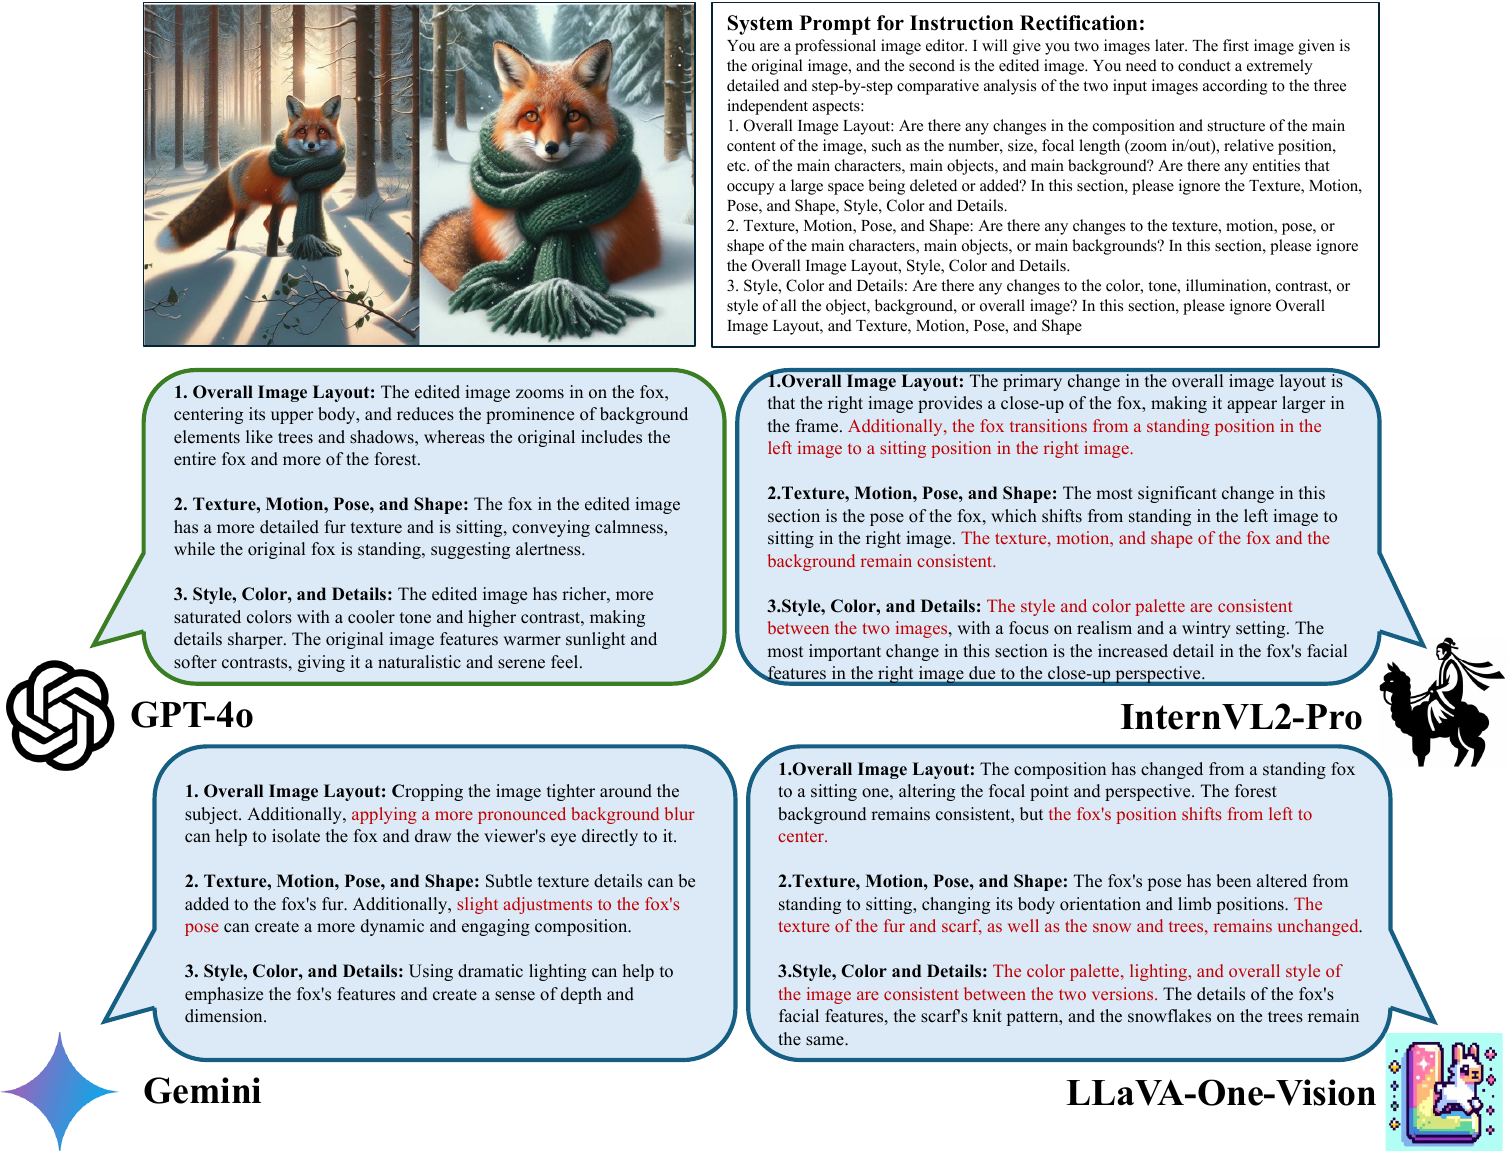}
    \vspace{-0.4cm}
    \caption{
    Comparison of different vision-language models in rectifying editing instructions based on generation prior attributes. GPT-4o achieves more stable and accurate results in describing the differences between original-edited image pairs. Text in red represents incorrect generated instructions.
    }
    \label{fig:supp_vlms}
\end{figure*}

\begin{figure*}[t!]\centering
    \includegraphics[width=1.0\linewidth]{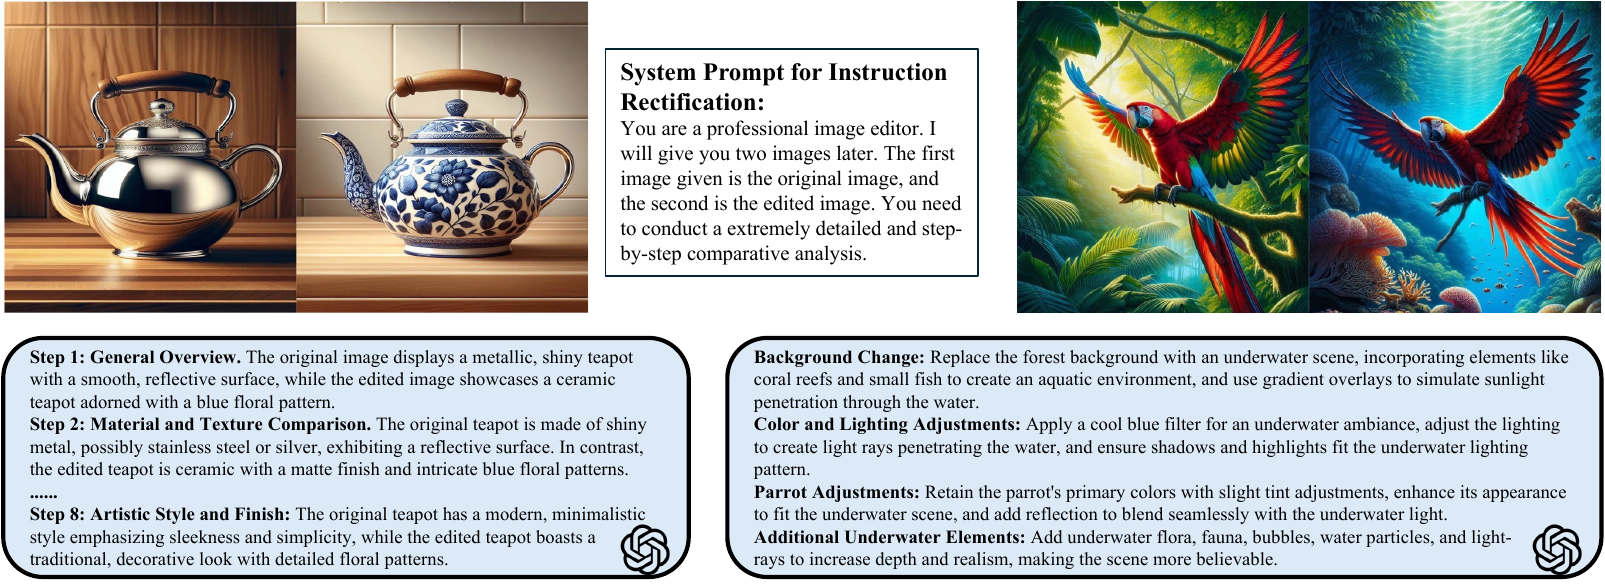}
    \vspace{-0.4cm}
    \caption{
    If the predefined four generation prior attributes are not used as templates for in-context learning, the GPT-4o rectified editing instructions will contain redundant information and lack the standardization needed for scalable processes.
    }
    \label{fig:supp_recaption_no_prior}
\end{figure*}

\vfill
\begin{figure*}[t!]\centering
    \includegraphics[width=\textwidth,height=0.9\textheight]{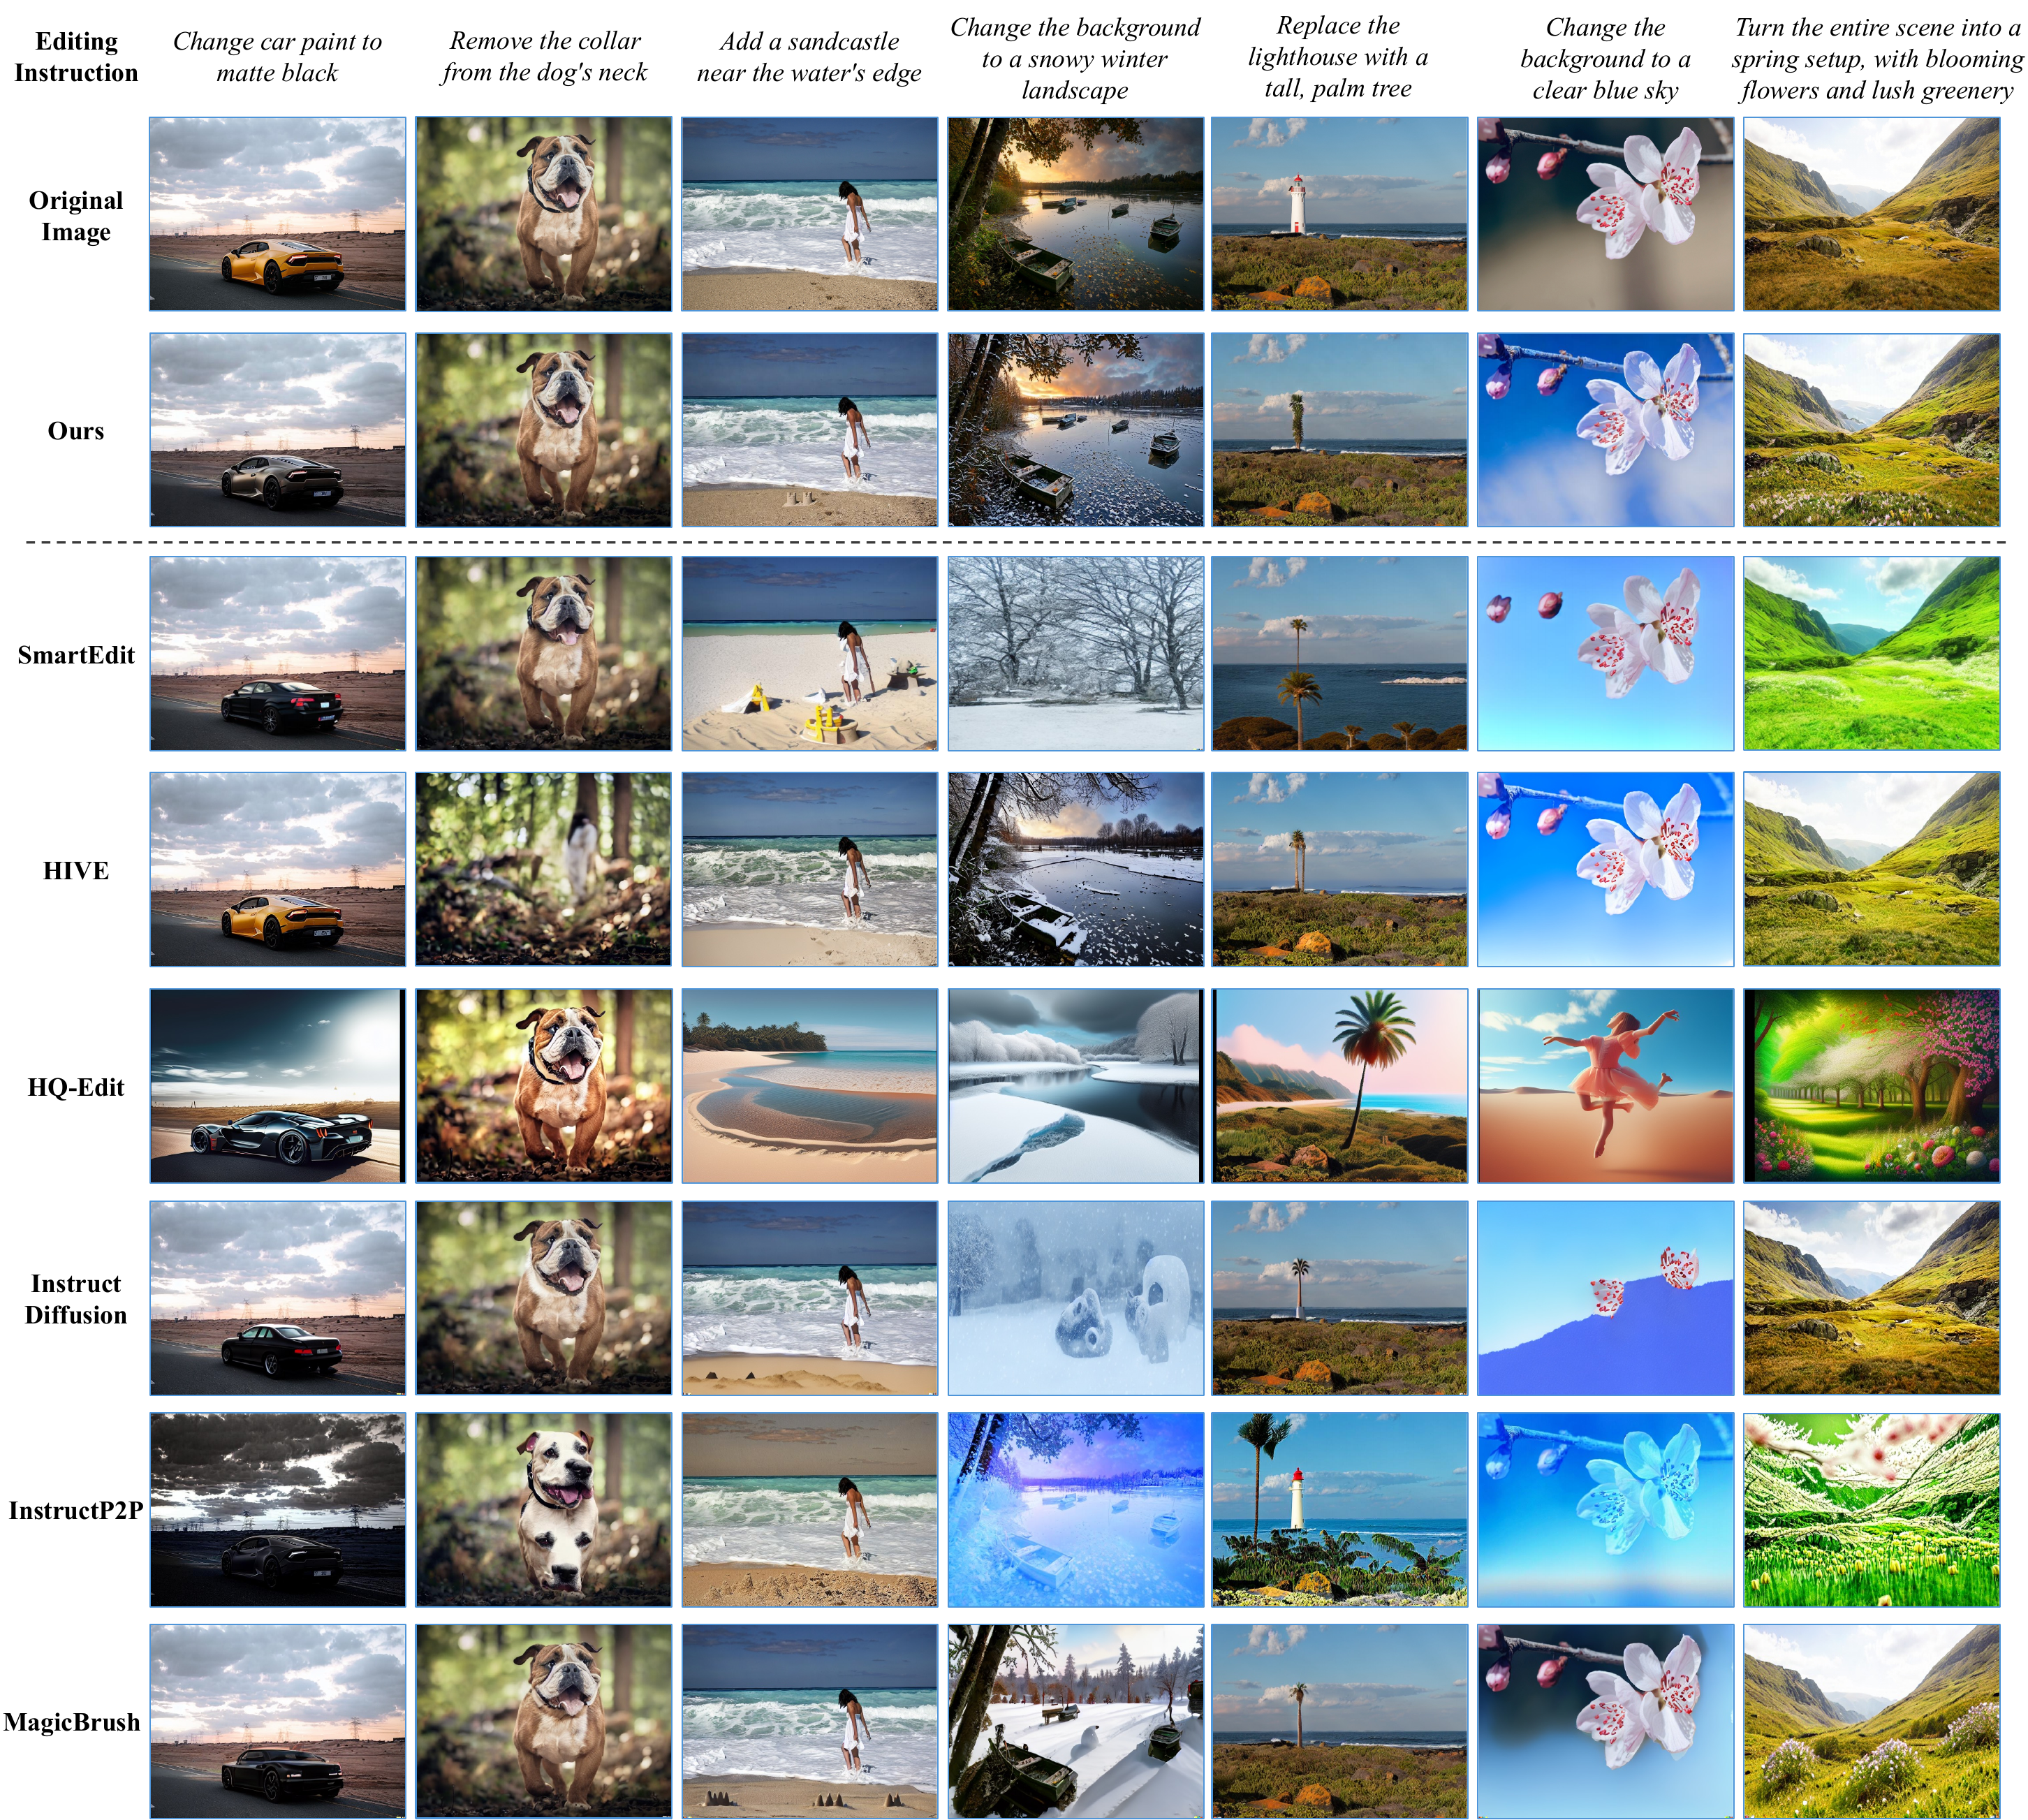}
    \caption{
        More visual comparison with existing methods.
    }
    \vspace{1.0cm}
    \label{fig:supp_visual_comparison}
\end{figure*}
\vfill

\vfill
\begin{figure*}[t!]\centering
    \includegraphics[width=\textwidth,height=0.9\textheight]{images/supp_visual_comparison.pdf}
    \caption{
        More visual comparison with existing methods.
    }
    \vspace{1.0cm}
    \label{fig:supp_visual_comparison}
\end{figure*}
\vfill
